# Supplementary material for: SkipCat: Rank-Maximized Low-Rank Compression of Large Language Models via Shared Projection and Block Skipping
Source: arXiv:2512.13494 source file (2026-10-27)
Supplement: Supplementary file 1 [file complexity.tex]

\section{Complexity}

\begin{table}[!htbp]
    \centering
    \begin{tabular}{c|c}
    \toprule
        & Time and Space Complexity \\
    \midrule
        Baseline  & $\mathcal{O} (Cd_{\mathrm{in}}d_{\mathrm{out}})$ \\
        Naïve  & $\mathcal{O} (Cr(d_{\mathrm{in}}+d_{\mathrm{out}}))$ \\
        Cat & $\mathcal{O} (r(d_{\mathrm{in}}+Cd_{\mathrm{out}}))$ \\
        Skip  & $\mathcal{O} (Cr(d_{\mathrm{in}}+d_{\mathrm{out}}-r))$ \\
        SkipCat  & $\mathcal{O} (r(d_{\mathrm{in}}+Cd_{\mathrm{out}}-r))$ \\
    \bottomrule
    \end{tabular}
    \caption{Time and memory complexity of standard weight multiplication (Baseline), its naïve low-rank approximation (Naïve), matrix concatenation (Cat), block skipping (Skip), and our proposed SkipCat. Here, $r$ denotes the rank, $d_{\mathrm{in}}$ and $d_{\mathrm{out}}$ are the input and output dimensions, respectively, and $C$ is the number of concatenated matrices. SkipCat reduces both floating‐point operations (FLOPs) and memory requirements compared to the other methods.}

    \label{tab:flops}
\end{table}

% \begin{table}[!htbp]
%     \centering
%     \begin{tabular}{c|cc}
%     \toprule
%         & FLOPs & \#Params \\
%     \midrule
%         Baseline  & $2d_{\mathrm{in}}d_{\mathrm{out}}$ & $d_{\mathrm{in}}d_{\mathrm{out}}$ \\
%         Naïve  & $2r(d_{\mathrm{in}}+d_{\mathrm{out}})$ & $r(d_{\mathrm{in}}+d_{\mathrm{out}})$ \\
%         Skip  & $2r(d_{\mathrm{in}}+2d_{\mathrm{out}}-r)+r$ & $r(d_{\mathrm{in}}+d_{\mathrm{out}}-r)$ \\
%     \bottomrule
%     \end{tabular}
%     \caption{Comparison of computational costs for standard weight multiplication (Baseline), its low-rank approximation (LR), and the proposed Schur method. The Schur method achieves fewer floating‐point operations (FLOPs) and a reduced parameter count compared to baseline and LR.}
%     \label{tab:flops2}
% \end{table}

% \input{tab}
